# Supplementary material for: Treant: Training Evasion-Aware Decision Trees
Source: arXiv:1907.01197 source file (2019-07-03)
Supplement: Supplementary file 1 [file appendix.tex]

\clearpage

\section{Dataset Information}
\label{app:datasets}
The \census\ dataset includes demographic information of $45,222$ US citizens, and the associated binary prediction task is to guess whether the yearly income of a person exceeds \$50,000 (positive) or not (negative). The class distribution on \census\ is moderately skewed, with approximately $75\%$ of the instances labeled as negative and the remaining $25\%$ as positive.
We therefore split the original dataset into two portions using stratified random sampling: a training set which accounts for $2/3$ of the total number of instances, and a test set containing the remaining $1/3$. Finally, each instance is described by a set of $13$ features, both numerical and categorical. 

The \wine\ dataset represents different types of wine based on the results of physio-chemical tests and the corresponding prediction task amounts to estimating quality on a scale from 0 to 10. For simplicity, we convert this task into a binary classification problem, where the positive class identifies good-quality wines (i.e., those whose quality is at least 6) and the negative class contains everything else. This dataset collects $6,497$ instances, each one represented by $12$ features ($11$ numerical plus $1$ dummy variable indicating whether the wine is white or not). The skewness of the class distribution here is less pronounced than that of \census, as about $63\%$ of the instances are labeled as positive and $37\%$ as negative. Still, we split the \wine\ dataset into two portions using stratified random sampling: a training set containing $80\%$ of the total number of instances, and a test set with the remaining $20\%$.
